# Supplementary material for: Non-adiabatic Storage of Short Light Pulses in an Atom-Cavity System
Source: arXiv:1903.10922 source file (2019-09-19)
Supplement: Supplementary file 1 [file SupplementalMaterial.pdf]

# Supplemental Material for "Non-adiabatic Storage of Short Light Pulses in an Atom–Cavity System"

Tobias Macha,* Eduardo Uruñuela, Wolfgang Alt, Maximilian Ammenwerth, Deepak Pandey, Hannes Pfeifer, and Dieter Meschede
*Institut für Angewandte Physik, Universität Bonn, Wegelerstraße 8, 53115 Bonn, Germany*

## EXPERIMENTAL METHODS

### Tripod Configuration

Here, we briefly explain the choice of the tripod configuration [S1].In our experiment, a few tens of neutral $^{87}$Rb atoms are trapped from the background gas ($10^{-10}$ mbar) and cooled in a magneto-optical trap, which is located 1 mm away from the cavity center. An optical lattice acting as a conveyor belt is used to transport them into the cavity region. Here, the presence of an atom is detected by its interaction with a near-resonant probe field at 780 nm, which is injected into the cavity via the HT mirror. This $\sigma^-$-polarized field drives the cycling transition $|F=2, m_F=-2\rangle \rightarrow |F'=3, m_F=-3\rangle$, which allows for a clean, non-destructive hyperfine state detection [S2]. In the presence of a continuous repumper, which prepares the atom in its $F=2$ ground state manifold, the atomic presence is detected by an increase of the reflected probe light and the transport is stopped. At the same time, probe and repumper also prepare the atom in $|F=2, m_F=-2\rangle$, the chosen initial state for the storage protocol.

However, mapping the population between the two ground states via a Raman process (Fig. 1c) has to involve the excited state $F'=2$ or $F'=1$, so as a next step, we change the cavity length such that its resonance frequency is shifted by 267 MHz. Then, the cavity mode is resonant with the $|F=2, m_F=-2\rangle \rightarrow |F'=2, m_F=-1\rangle$ transition, which is driven by the weak coherent light pulse. In the shifting process, we also measure the vacuum Rabi splitting [S3], from which we infer the atom-cavity coupling strength for each individual atom, see Figure S.1a.

To make use of these well-established techniques for our experiment [S4], the tripod configuration emerged as a first choice for the demonstration of short light pulse storage. However, for quantum memory applications it is not ideal. Our experiment therefore is a proof-of-principle for high bandwidth applications and a milestone in the agreement between expected and measured efficiencies.

Besides that, the tripod configuration also opens new possibilities, since every photon generation attempt creates entanglement between the emitted photon and the magnetic sublevels of the atom, which is e.g. useful for teleportation experiments [S5] or the generation of entanglement between different platforms [S6]. In [S7], the properties of such a system are investigated and the creation of two-mode Schrödinger-cat states in the cavity is proposed.

### Single-Photon Generation

For generating single photons, we make use of an adiabatic two-photon Raman process known as vSTIRAP [S8]. The probability of receiving more than one photon per read pulse and emitter is practically zero, since the excitation laser frequency is far-detuned from the emission frequency. But in order to identify the presence of more than one atom in the cavity mode, it is interesting to analyze the normalized cross-correlation $g_c^{(2)}(\Delta x)$ between photon detections in SPCM 1 and 2 of the Hanbury Brown-Twiss setup. If the individual SPCM $i$ sees $c_i$ counts in the 100 ns generation window $x$, $g_c^{(2)}$ is defined as:

$$g_c^{(2)}(\Delta x) = \frac{1}{\overline{m}} \frac{\langle c_1(x)\, c_2(x+\Delta x)\rangle}{\langle c_1(x)\rangle \langle c_2(x)\rangle}, \qquad \text{(S.1)}$$

where $\overline{m}$ is the average number of coincidences for $\Delta x \neq 0$.

In Figure S.1b, we show the detection coincidences for a shift of $\Delta x$ windows along with the Poissonian error given by the number of coincidences. At $\Delta x = 0$, the dip is expected to reach zero for a perfect single-photon source [S9, S10], but it is usually limited by the dark count rates of the SPCMs and by Raman-scattered lock laser light [S11]. These two effects are combined into the rates $x_{d_1} = (3.00\pm0.03)$ kcps and $x_{d_2} = (1.20\pm0.01)$ kcps in order to give the estimate

$$g_{c,bg}^{(2)}(0) \approx \frac{\eta_{retrieval}\,(x_{d_1}+x_{d_2})}{(\eta_{retrieval}/2 + x_{d_1})\,(\eta_{retrieval}/2 + x_{d_2})} = (13.6 \pm 0.1)\ \%,$$

which is derived from Equation S.1 for equal SPCM detection efficiencies and the probability of detecting a photon per triggered pulse $\eta_{retrieval} = (2.3\pm0.1)$ %. For all $g$-values in Figure S.1a we find $g_c^{(2)}(0) = (20.9 \pm 3.4)$ %, which means the contrast is not background limited, but most likely constrained by a small two-atom component. In order to filter the spurious events, we post-select the data for $g \in [70, 80] \cdot 2\pi$ MHz (highlighted in

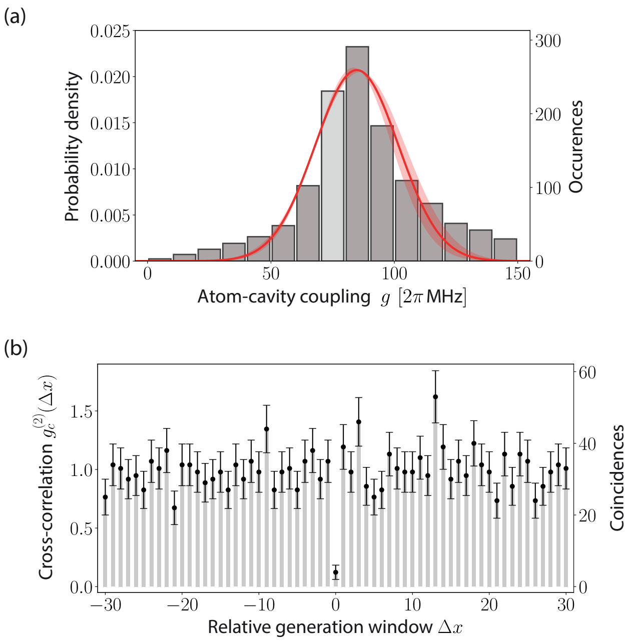


FIG. S.1. **(a)** The vacuum-Rabi splitting is measured to determine the individual atom-coupling strength $g$ for each sequence repetition. The distribution of values is shown with a Gaussian fit and $1\sigma$ confidence intervals. Each value still has to be scaled by $\sqrt{1/6}$ to obtain the coupling strength on the $|2,-2\rangle \rightarrow |2',-1\rangle$ transition. As discussed in the main text, a specified range of coupling strengths (highlighted area) is used for post-selection in (b) and for an accurate implementation of $g$ in our simulations. **(b)** The cross-correlation $g_c^{(2)}$ of detected photons according to Equation S.1 reveals $g_c^{(2)}(0) = (12.2 \pm 6.5)$ %, if post-selection with $g \in [70, 80] \cdot 2\pi$ MHz is applied. In this case, only single atoms are present. As our correlation is limited to $g_{c,bg}^{(2)}(0) \approx (13.6 \pm 0.1)$ % by detector dark- and background counts, the measurement confirms that our system indeed delivers single photons.

Fig. S.1b). As can be seen from Figure S.1b, the value $g_c^{(2)}(0) = (12.2 \pm 6.5)$ % is then close to the background limit, as expected. The bottleneck for giving precise $g_c^{(2)}(0)$ estimates is the number of measurements.

## THEORETICAL MODEL

### A Coherently Driven Multi–Level Atom in a Dissipative Cavity

First, we start with the more intuitive scenario of a closed system: The well-known Jaynes-Cummings Hamiltonian [S12] describes the interaction between two atomic levels and a quantized mode of an electromagnetic field. We first extend this model to a three-level atom with two ground states $|g_1\rangle, |g_2\rangle$ and one excited state $|e\rangle$, where only the transition from $|g_2\rangle \rightarrow |e\rangle$ with frequency $\omega_{a_2}$ is resonant with the cavity. The Hamiltonian of this atom-cavity system consists of several parts:

$$\hat{H}_{\mathrm{JC}} = \hat{H}_{\mathrm{a}} + \hat{H}_{\mathrm{c}} + \hat{H}_{\mathrm{int}}\,,$$

where $\hat{H}_{\mathrm{a}}$ and $\hat{H}_{\mathrm{c}}$ are the separate Hamiltonians of atom and cavity mode, while $\hat{H}_{\mathrm{int}}$ describes the interaction.

We treat the atom-photon interaction in both dipole- and rotating-wave approximations, and simplify the individual Hamiltonians by putting the dynamics in the frame of the pulse and Raman laser with frequencies $\omega_{\mathrm{p,R}}$. The atom energy in the presence of a single-photon detuning $\Delta_{\text{p-a}} = \omega_{\mathrm{p}} - \omega_{a_2}$ with respect to the excited state and a two-photon detuning $\delta = \Delta_{\text{p-a}} - (\omega_{\mathrm{R}} - \omega_{a_1})$ with respect to the ground state $|g_1\rangle$ is given by:

$$\hat{H}_{\mathrm{a}} = -\hbar\,\Delta_{\text{p-a}} \cdot \hat{\sigma}_{ee} - \hbar\,\delta \cdot \hat{\sigma}_{g_1 g_1}\,. \qquad \text{(S.2)}$$

We introduce the raising and lowering operators $\sigma_{kl}^{\dagger} = |l\rangle\langle k|$ and $\sigma_{kl} = |k\rangle\langle l|$ which describe the excitation and de-excitation of the atomic spin, respectively.

The energy of the cavity field can be expressed in analogy to the spectrum of a harmonic oscillator by $m$ Fock states $|0\rangle, ..., |m\rangle$. The creation- and annihilation operators $\hat{a}^{\dagger}$ and $\hat{a}$ add or remove a photon from the cavity mode with resonance frequency $\omega_c$, so that its energy for a certain frequency detuning between input pulse and cavity resonance $\Delta_{\text{p-c}} = (\omega_c - \omega_{a_2}) - \Delta_{\text{p-a}} = \Delta_{\text{c-a}} - \Delta_{\text{p-a}}$ reads:

$$\hat{H}_{\mathrm{c}} = -\hbar\,\Delta_{\text{p-c}} \cdot \hat{a}^{\dagger}\hat{a}\,.$$

In the following, we consider the special case $\Delta_{\text{p-c}} = \Delta_{\text{p-a}} = \delta = 0$.

The interaction term describes the coupling between the atomic dipole and the electric field of the cavity mode, which occurs with the Rabi frequency $2g$:

$$\hat{H}_{\mathrm{int}} = i\,\hbar\,g\left(\hat{\sigma}_{g_2 e}^{\dagger}\hat{a} - \hat{\sigma}_{g_2 e}\,\hat{a}^{\dagger}\right)\,. \qquad \text{(S.3)}$$

We extend this model by two coherent, time-dependent driving terms, for which the overall Hamiltonian $\hat{H}(t)$ is given by

$$\hat{H}(t) = \hat{H}_{\mathrm{JC}} + \hat{H}_{\mathrm{d}}(t)\,, \qquad \text{(S.4)}$$

with the driving Hamiltonian

$$\hat{H}_{\mathrm{d}}(t) = i\,\hbar\,\frac{\Omega(t)}{2}\left(\hat{\sigma}_{g_1 e}^{\dagger} - \hat{\sigma}_{g_1 e}\right) + \hbar\,\mathcal{E}(t)\left(\hat{a}^{\dagger} + \hat{a}\right)\,. \qquad \text{(S.5)}$$

The first term with $\Omega(t)$ stands for the control laser-induced interaction in a $\Lambda$-configuration. The control laser addresses the transition from ground to excited state, which is not coupled to the cavity. The second term populates the cavity mode according to the driving strength $\mathcal{E}(t)$.

Without dissipative processes, i.e. the interaction of our system with the environment, we cannot fully control the ground state population of our system, as is intuitively clear from Equations S.5 and S.3: Any excitations brought into the system would lead to infinite oscillations between the states $|g_2\rangle$ and $|e\rangle$ as soon as the control laser does not realize a full population transfer to $|g_1\rangle$. The environmental states on the other hand are unknown, so we introduce the density matrix formalism and 'open' our system to loss channels. The Schrödinger equation is replaced by the master equation [S13], which describes the density matrix $\hat{\rho}$ of our closed system at any point in time:

$$\frac{d\hat{\rho}}{dt} = \hat{\mathcal{L}}\,\hat{\rho} = -\frac{i}{\hbar}\left[\hat{H},\hat{\rho}\right] + \sum_l \hat{\mathcal{C}}_l\hat{\rho}\hat{\mathcal{C}}_l^\dagger - \frac{1}{2}\left(\hat{\mathcal{C}}_l^\dagger\hat{\mathcal{C}}_l\hat{\rho} + \hat{\rho}\hat{\mathcal{C}}_l^\dagger\hat{\mathcal{C}}_l\right) . \tag{S.6}$$

The Liouvillian super-operator $\hat{\mathcal{L}}$ contains both the coherent dynamics given by Equation S.4 and the Lindblad terms attributed to the decay and loss channels, which are specified by the collapse operators $\hat{\mathcal{C}}_l$:

$$\hat{\mathcal{C}}_{\gamma_1} = \sqrt{2\gamma_1}\,\hat{\sigma}_{g_1,e} \;\;,\;\; \hat{\mathcal{C}}_{\gamma_2} = \sqrt{2\gamma_2}\,\hat{\sigma}_{g_2,e} \;\;, \quad \hat{\mathcal{C}}_{\kappa} = \sqrt{2\kappa}\,\hat{a}\,. \tag{S.7}$$

The transmission rate $\kappa_{\rm HT}$ through the HT mirror and the unwanted damping of the field due to absorption, scattering at the mirrors and leakage through the LT mirror at rate $\kappa_{\rm loss}$ form the total cavity loss rate $\kappa = \kappa_{\rm HT} + \kappa_{\rm loss}$. The excited state decay $\Gamma = 2\gamma$ to both ground states is considered with independent rates $\gamma_{1,2}$ such that $\gamma = \gamma_1 + \gamma_2$.

The conversion of modes on the outside of a resonator to modes on the inside is commonly treated by the *input-output formalism* [S14, S15]. For mapping a weak coherent pulse with electric field probability amplitude $\phi_{\rm in}(t)$ into the atom, we have to express the driving term $\mathcal{E}(t)$ in terms of $\phi_{\rm in}(t)$ which contains on average $n$ photons:

$$\mathcal{E}(t) = \sqrt{2\kappa_{\rm HT}}\cdot\sqrt{n}\cdot\phi_{\rm in}(t)\,. \tag{S.8}$$

Here, we have considered that $\phi_{\rm in}(t)$ has a temporal shape of length $T$, to which it is normalized such that $\int|\phi_{\rm in}(t)|^2\,dt = 1$, and a mean number of photons $n$. For a given $\phi_{\rm in}(t)$ in the adiabatic storage regime, $\Omega(t)$ is found according to [S16].

In summary, our model now describes the temporal evolution of an idealized, three-level atom coupled to a resonator, including losses as well as driven excitations. We can extract information, e.g. about the average intracavity photon number $\overline{n} = \langle\hat{a}^\dagger\hat{a}\rangle$ at any point in time. In the case of single-photon generation, the simulation provides predictions for $\mathcal{E}(t) = 0$. For our simulation plots, we solve Equation S.6 to investigate the efficiency of coherent-pulse storage in dependence of its various parameters. For $t > T$, the system reaches a steady state ($\hat{\mathcal{L}}\,\hat{\rho} = 0$), which allows us to define the storage efficiency $\eta_{\rm storage}$ by the atomic state population in $|g_1\rangle$:

$$\eta_{\rm storage} = \frac{\rho_{g_1g_1}}{n} = \frac{\langle\hat{\sigma}^\dagger_{g_1g_1}\hat{\sigma}_{g_1g_1}\rangle}{n}\,. \tag{S.9}$$

Leaving the regime of weak coherent pulses with on average one photon ($n = 1$), we explore the dynamics in the limit $n \ll 1$. Remarkably, the results for $\eta_{\rm storage}$ then correspond exactly to the predictions for single-photon Fock-state storage in [S16, S17]: In the adiabatic storage regime of $TC\gamma \gg 1$, the storage efficiency is limited to:

$$\eta_{\rm max} = \frac{C}{C+1}\,, \tag{S.10}$$

where $C = \frac{g^2}{\kappa\,\gamma}$ is the cooperativity parameter.

In [S18], the - to our knowledge most recent - model to describe single-photon storage is complex, as it involves the coupling of several electromagnetic modes inside and outside the resonator. Here, the excited state decay is directed to an auxiliary state outside the three-level atom, most likely to quantify the free-space loss. The main new aspect of their work is an analysis of the drop in efficiency caused by *parasitic losses* ($\kappa_{\rm loss}$). In their presence, a new limit for the optimum storage efficiency is found:

$$\eta'_{\rm max} = \frac{\kappa}{\kappa+\kappa_{\rm loss}}\frac{C'}{C'+1}\,, \tag{S.11}$$

where $C' = \frac{g^2}{(\kappa+\kappa_{\rm loss})\,\gamma}$ is the loss-modified cooperativity. For $\kappa_{\rm loss} \neq 0$, we obtain efficiencies according to S.11 as well. Also, in our model the population sum in all coherently coupled states is conserved, which is a more realistic case when considering adiabatic storage processes.

### A Four–Level Atom Coupled to Two Cavity Modes

In our tripod configuration, the mediating atomic excited state is coupled to two $\sigma^\pm$ cavity modes. This means an additional state $|g_3\rangle$ of approximately equal energy as $|g_2\rangle$ has to be taken into account (see Fig. 1c of the main text). The corresponding operators acting on the photon number in the second cavity mode are $\hat{b}^\dagger$ and $\hat{b}$. Thus we modify the interaction Hamiltonian in Equation S.3 and the collapse operators in Equation S.7 to

$$\hat{H}'_{\rm int} = i\,\hbar\,g\left(\hat{\sigma}^\dagger_{g_2e}\hat{a} - \hat{\sigma}_{g_2e}\,\hat{a}^\dagger\right) + i\,\hbar\,g'\left(\hat{\sigma}^\dagger_{g_3e}\hat{b} - \hat{\sigma}_{g_3e}\,\hat{b}^\dagger\right) \tag{S.12}$$

and

$$\hat{\mathcal{C}}'_{\gamma'_1} = \sqrt{2\gamma'_1}\,\hat{\sigma}_{g_1,e} \;\;,\;\; \hat{\mathcal{C}}'_{\gamma'_2} = \sqrt{2\gamma'_2}\,\hat{\sigma}_{g_2,e} \;\;, \quad \hat{\mathcal{C}}'_{\gamma_3} = \sqrt{2\gamma_3}\,\hat{\sigma}_{g_3,e} \;\;,\;\; \hat{\mathcal{C}}'_{\kappa_a} = \sqrt{2\kappa}\,\hat{a} \;\;,\;\; \hat{\mathcal{C}}'_{\kappa_b} = \sqrt{2\kappa}\,\hat{b}\,,$$

with the new coupling strength $g'$ and an adjusted branching ratio of the excited state decays $\gamma_3$ and $\gamma'_{1,2}$. In reality, there are more levels to decay to, but their respective transitions strengths are weak, such that we may neglect them. Additionally, the excited state population decay is very small at any time ($\kappa \gg \gamma_i$).

The cooperativity parameter $C$ is defined for a single atom-cavity coupling rate only. We are not aware of any generalized rate depending on $g$ and $g'$, so we cannot estimate the efficiency as in S.11. Instead, we only give results based on our simulations.

### Multilevel Atoms

We assume transform-limited pulses, i.e. for our given pulse duration and shape, a minimum spectral width is implied. As a consequence, the real multilevel character of atoms has to be taken into account. For $^{87}$Rb, the Raman laser addressing the $|F=1, m_F=-1\rangle \rightarrow |F'=2, m_F=-1\rangle$ transition has a non-zero probability of driving the $\Delta = 157$ MHz red-detuned $|F=2, m_F=-2\rangle \rightarrow |F'=1, m_F=-1\rangle$ transition, which is why the state $|f\rangle = |F'=1, m_F=-1\rangle$ should be taken into account. The cavity itself acts as a frequency filter for the input pulse, reducing the probability for off-resonant transitions to less than relative 2.5 %.

In our simulation we include multilevel-atom effects by introducing the detuned excited state with energy

$$\hat{H}_\mathrm{a} = -\hbar\,\Delta \cdot \hat{\sigma}_{ff} \tag{S.13}$$

and extending Equation S.5 to

$$\begin{aligned}\hat{H}'_\mathrm{d}(t) = \quad & i\,\hbar\,\frac{\Omega(t)}{2}\left(\hat{\sigma}^\dagger_{g_1 e} - \hat{\sigma}_{g_1 e}\right) + \hbar\,\mathcal{E}(t)\left(\hat{a}^\dagger + \hat{a}\right) \\ & + i\,\hbar\,\frac{\Omega'(t)}{2}\left(\hat{\sigma}^\dagger_{g_1 f} - \hat{\sigma}_{g_1 f}\right)\end{aligned}$$

and Equation S.12 to

$$\begin{aligned}\hat{H}''_\mathrm{int} =& i\,\hbar\,g\left(\hat{\sigma}^\dagger_{g_2 e}\hat{a} - \hat{\sigma}_{g_2 e}\,\hat{a}^\dagger\right) + i\,\hbar\,g'\left(\hat{\sigma}^\dagger_{g_3 e}\hat{b} - \hat{\sigma}_{g_3 e}\,\hat{b}^\dagger\right) \\ & + i\,\hbar\,g''\left(\hat{\sigma}^\dagger_{g_2 f}\hat{a} - \hat{\sigma}_{g_2 f}\,\hat{a}^\dagger\right) + i\,\hbar\,g'''\left(\hat{\sigma}^\dagger_{g_3 f}\hat{b} - \hat{\sigma}_{g_3 f}\,\hat{b}^\dagger\right),\end{aligned}$$

where $\Omega'(t)$, $g''$ and $g'''$ are the new coupling strengths obtained by the ratio of Clebsch-Gordan coefficients. The decay rates and collapse operators are adjusted as well. This is finally the model we use to interpret our measured data.

The main effect of an additional excited state $|1', -1\rangle$ is that a small fraction of the population in the target state $|1, -1\rangle$ is transferred to the excited state and back during the storage process. These dynamics result in a slightly reduced expected efficiency compared to a simplified four-level atom approach. However, for well-controlled polarizations of the manipulating beams and

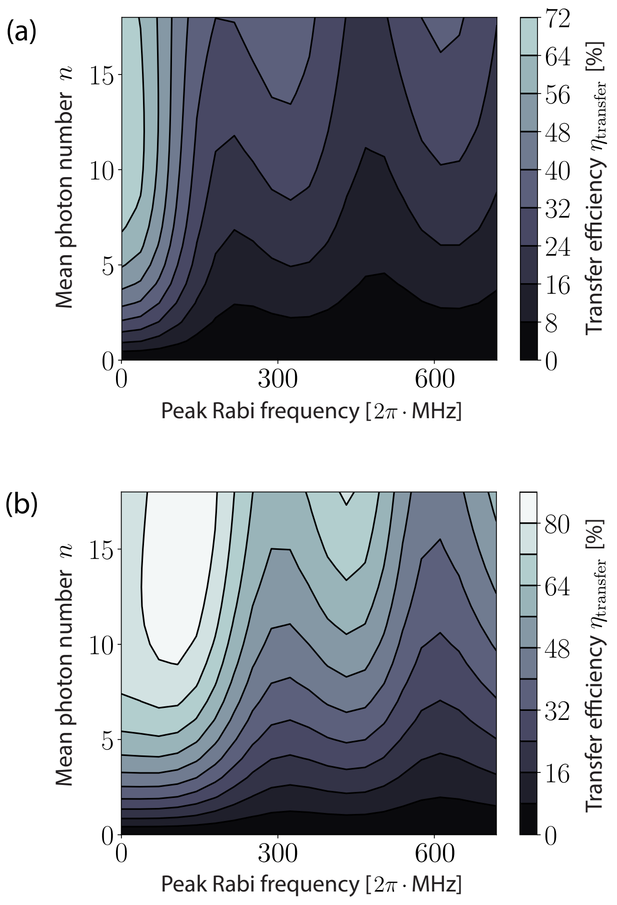


FIG. S.2. Figure 3b of the main text shows the population transfer $\eta_\mathrm{transfer}$ to $|F, m_F\rangle = |1, -1\rangle$ as a function of the mean input pulse photon number $n$ and the control pulse peak Rabi frequency. Here, plot **(a)** shows the transfer to $|2, 0\rangle$, while plot **(b)** displays the sum of the transfer efficiencies to both states. The total transfer reaches above 80 %, in agreement with the expectation for large $n$.

cavity modes, five states are sufficient to describe a real multilevel-atom, since the $F' = 3$ level does not couple to the target ground state. Additionally, it is not addressed by the input pulse, which is frequency-filtered by the cavity.

### On the Maximum Achievable Transfer Efficiency

In Figure 3b, the maximum achievable transfer efficiency is limited to slightly above 60 %, even for high input photon numbers. The transfer efficiency only regards transfer to $|1, -1\rangle$ and neglects the population in the undesired state $|2, 0\rangle$. In Figure S.2 the transfer to $|2, 0\rangle$ is shown, as well as the sum of the transfers to both states. The combined transfer reaches above 80 %, a value which might converge towards 100 % for even higher mean photon numbers [S19]. However, simulations for several tens

of Fock states and a five-level atom are computationally challenging. Intuitively it is clear that cavity field dampings due to both $\kappa_{\text{loss}}$ and $\kappa_{\text{HT}}$ can be compensated by sending larger input fields. But the coherent population leakage in a tripod configuration will always take place, reducing the efficiency of transfer to the target state.

## Numerical Tools

Exact analytical solutions to the master equation S.6 are only possible in special cases. In general, a numerical approach is the easier choice. We use *QuTiP* (v4.1), the *Quantum Toolbox in Python* (v3.5) [S20, S21] to facilitate the process of setting up state vectors, time-(in)dependent Hamiltonians and (super-)operators and to solve Equation S.6 with the in-built function *mesolve*. Based on an ordinary differential equation solver, it evolves the density matrix and returns a time-binned array of expectation values for a list of operators. As a result, for example the shape of generated photons can be simulated:

In order to fit these shapes and to obtain the system parameters, we developed our own optimal control scheme based on *basin-hopping*. Basin-hopping [S22] is a stochastic algorithm which is similar to the well-known *Simulated Annealing* (SA) algorithm. As opposed to gradient-based search algorithms, it is less liable to end up in a local minimum while determining the global minimum of a cost function in a large parameter space.

The algorithm iterates through cycles composed of random perturbation of the parameters, local optimization by a routine to be specified and acceptance or rejection of the parameter set $P$ based on the cost function value. We apply the *Nelder-Mead method* [S23], also known as *downhill simplex method*, for the local optimization. Based on the concept of simplices, it approximates local optima by evaluating cost values along the $P+1$ points of a volume and introducing variations such that the cost value decreases. For fitting the photon shape, we define the cost function $\mathcal{C}_{\text{retrieval}}$ as:

$$\mathcal{C}_{\text{retrieval}} = \overline{n}_{\text{exp}}(t) - n_0 \cdot \overline{n}\left(t, \tau_\Omega, \Omega(t), \Delta, g_{\text{dist}}\right) , \quad \text{(S.14)}$$

where the average photon number $\overline{n}(t)$ given by the simulation depends on the mean value of $\Delta = \Delta_{\text{p-a}}$ and the driving Rabi frequency $\Omega(t)$ and its pulse delay $\tau_\Omega$. The experimentally determined variation in coupling strengths is implemented as a distribution $g_{\text{dist}}$ (as in Fig. S.1a), over which we average along with the different initial $m_F$ ground states. $\overline{n}$ is scaled with $n_0$ in order to reduce the difference of $\overline{n}(t)$ and the measured average detector counts $\overline{n}_{\text{exp}}(t)$. Once the simulation finds the parameters to recreate $\overline{n}_{\text{exp}}(t)$, we can estimate the efficiency of photon generation by the population sum of the $F=2$ states $(\rho_{g_2g_2} + \rho_{g_3g_3})$ in the steady state.

* macha@iap.uni-bonn.de

[S1] N. V. Vitanov, A. A. Rangelov, B. W. Shore, and K. Bergmann, Reviews of Modern Physics **89**, 015006 (2017).
[S2] R. Gehr, J. Volz, G. Dubois, T. Steinmetz, Y. Colombe, B. L. Lev, R. Long, J. Estève, and J. Reichel, Physical Review Letters **104**, 203602 (2010).
[S3] A. Boca, R. Miller, K. M. Birnbaum, A. D. Boozer, J. McKeever, and H. J. Kimble, Physical Review Letters **93**, 233603 (2004).
[S4] J. Gallego, W. Alt, T. Macha, M. Martinez-Dorantes, D. Pandey, and D. Meschede, Physical Review Letters **121**, 173603 (2018).
[S5] C. Nölleke, A. Neuzner, A. Reiserer, C. Hahn, G. Rempe, and S. Ritter, Physical Review Letters **110**, 140403 (2013).
[S6] M. Lettner, M. Mücke, S. Riedl, C. Vo, C. Hahn, S. Baur, J. Bochmann, S. Ritter, S. Dürr, and G. Rempe, Physical Review Letters **106**, 210503 (2011).
[S7] M. W. Janowicz and J. M. A. Ashbourn, Physical Review A **55**, 2348 (1997).
[S8] M. Mücke, J. Bochmann, C. Hahn, A. Neuzner, C. Nölleke, A. Reiserer, G. Rempe, and S. Ritter, Physical Review A **87**, 063805 (2013).
[S9] H. J. Kimble, M. Dagenais, and L. Mandel, Physical Review Letters **39**, 691 (1977).
[S10] H. Paul, Reviews of Modern Physics **54**, 1061 (1982).
[S11] J. Gallego, S. Ghosh, S. K. Alavi, W. Alt, M. Martinez-Dorantes, D. Meschede, and L. Ratschbacher, Applied Physics B **122**, 47 (2016).
[S12] E. Jaynes and F. Cummings, Proceedings of the IEEE **51**, 89 (1963).
[S13] H. J. Carmichael, *Statistical Methods in Quantum Optics 1: Master Equations and Fokker-Planck Equations* (Springer, 2002).
[S14] D. F. Walls and G. J. Milburn, *Quantum optics* (Springer Science & Business Media, 2007).
[S15] M. Aspelmeyer, T. J. Kippenberg, and F. Marquardt, Reviews of Modern Physics **86**, 1391 (2014).
[S16] J. Dilley, P. Nisbet-Jones, B. W. Shore, and A. Kuhn, Physical Review A **85**, 023834 (2012).
[S17] A. V. Gorshkov, A. André, M. D. Lukin, and A. S. Sørensen, Physical Review A **76**, 033804 (2007).
[S18] L. Giannelli, T. Schmit, T. Calarco, C. P. Koch, S. Ritter, and G. Morigi, New Journal of Physics **20**, 105009 (2018).
[S19] We have confirmed this behavior in the adiabatic regime for a lambda configuration.
[S20] J. Johansson, P. Nation, and F. Nori, Computer Physics Communications **184**, 1234 (2013).
[S21] J. Johansson, P. Nation, and F. Nori, Computer Physics Communications **183**, 1760 (2012).
[S22] D. Wales, *Energy landscapes: Applications to clusters, biomolecules and glasses* (Cambridge University Press, 2003).
[S23] F. Gao and L. Han, Computational Optimization and Applications **51**, 259 (2012).
